# Supplementary material for: detrex: Benchmarking Detection Transformers
Source: arXiv:2306.07265 source file (2023-06-13)
Supplement: Supplementary file 1 [file 08_appendix.tex]

\section{Appendix}

\begin{table*}[ht]
\centering\setlength{\tabcolsep}{7pt}

\footnotesize
\caption{{Supported detection transformer models of different codebases}}
\vspace{-0mm}
\resizebox{0.6\columnwidth}{!}{%
\begin{tabular}{lccc}
\shline
Model & detrex & MMdetection3.0 & Detectron2 \\
\shline
DETR & \cmark  & \cmark  & \cmark \\
Deformable-DETR  & \cmark & \cmark \\
Conditional-DETR  & \cmark &  \cmark \\
Anchor-DETR & \cmark & \\
PnP-DETR  & \cmark & \\
DAB-DETR  & \cmark & \cmark \\
DAB-Deformable-DETR  & \cmark & \\
DN-DETR  & \cmark & \\
DN-Deformable-DETR  &  \cmark & \\
DINO  & \cmark &  \cmark \\
Group-DETR & \cmark & \\
$\mathcal{H}$-DETR & \cmark & \\
DETA & \cmark & \\
Stable-DINO & \cmark & \\
MaskDINO & \cmark & \\
Lite-DETR & \cmark & \\
EDPose & \cmark & \\
\shline
\end{tabular}
\label{tab:compare_with_swin_backbone}}
\end{table*}

\begin{table*}[ht]
\centering\setlength{\tabcolsep}{7pt}

\footnotesize
\vspace{-0mm}
{
\resizebox{1.0\textwidth}{!}{%
\begin{tabular}{l|l|l|l|cccccc|c|c|c|c|c}
\shline
Backbone & Pretrained & Feature Scales & \#epochs  & AP & AP$_{50}$ & AP$_{75}$ & AP$_{S}$ & AP$_{M}$ & AP$_{L}$ & \#params & GFLOPs & FPS & Memory & GPU Hours \\
\shline
R50 & ImageNet1K & 5 & 12  & $49.6$ & 67.1 & 54.2 & 32.9 & 52.4 & 63.7 & 48.0M & & & 32.9GB & 116h\\
Swin-Large & ImageNet22K & 5 & 12  & $57.5$ & 75.9 & 63.1 & 39.9 & 61.0 & 73.5 & 218.3M & & & 61.4GB & 224h \\
Swin-Large & ImageNet22K & 5 & 36  & $58.5$ & 77.0 & 64.1 & 41.4 & 62.3 & 74.0 & 218.3M & & & 61.4GB & 468h\\
Focal-Large-4level & ImageNet22K & 5 & 12  & $58.5$ & 76.8 & 64.2 & 42.2 & 62.0 & 74.1 & 228.9M & & & 67.9GB & 186h \\
ConvNeXt-Large & ImageNet22K & 5 & 12  &  &  &  &  &  &  &  & & &  &  \\
InternImage-Large & ImageNet22K & 5 & 12  &  &  &  &  &  &  &  & & &  &  \\
\shline
\end{tabular}}
\vspace{-0.2cm}
\caption{The effective of DINO-5scale based on various backbones.}
\vspace{0.2cm}
\label{tab:benchmark_backbone_on_dino_5scale}
}
\end{table*}

\begin{figure}[h]
    \centering
    % \vspace{-0.2cm}
    \includegraphics[width=0.98\linewidth]{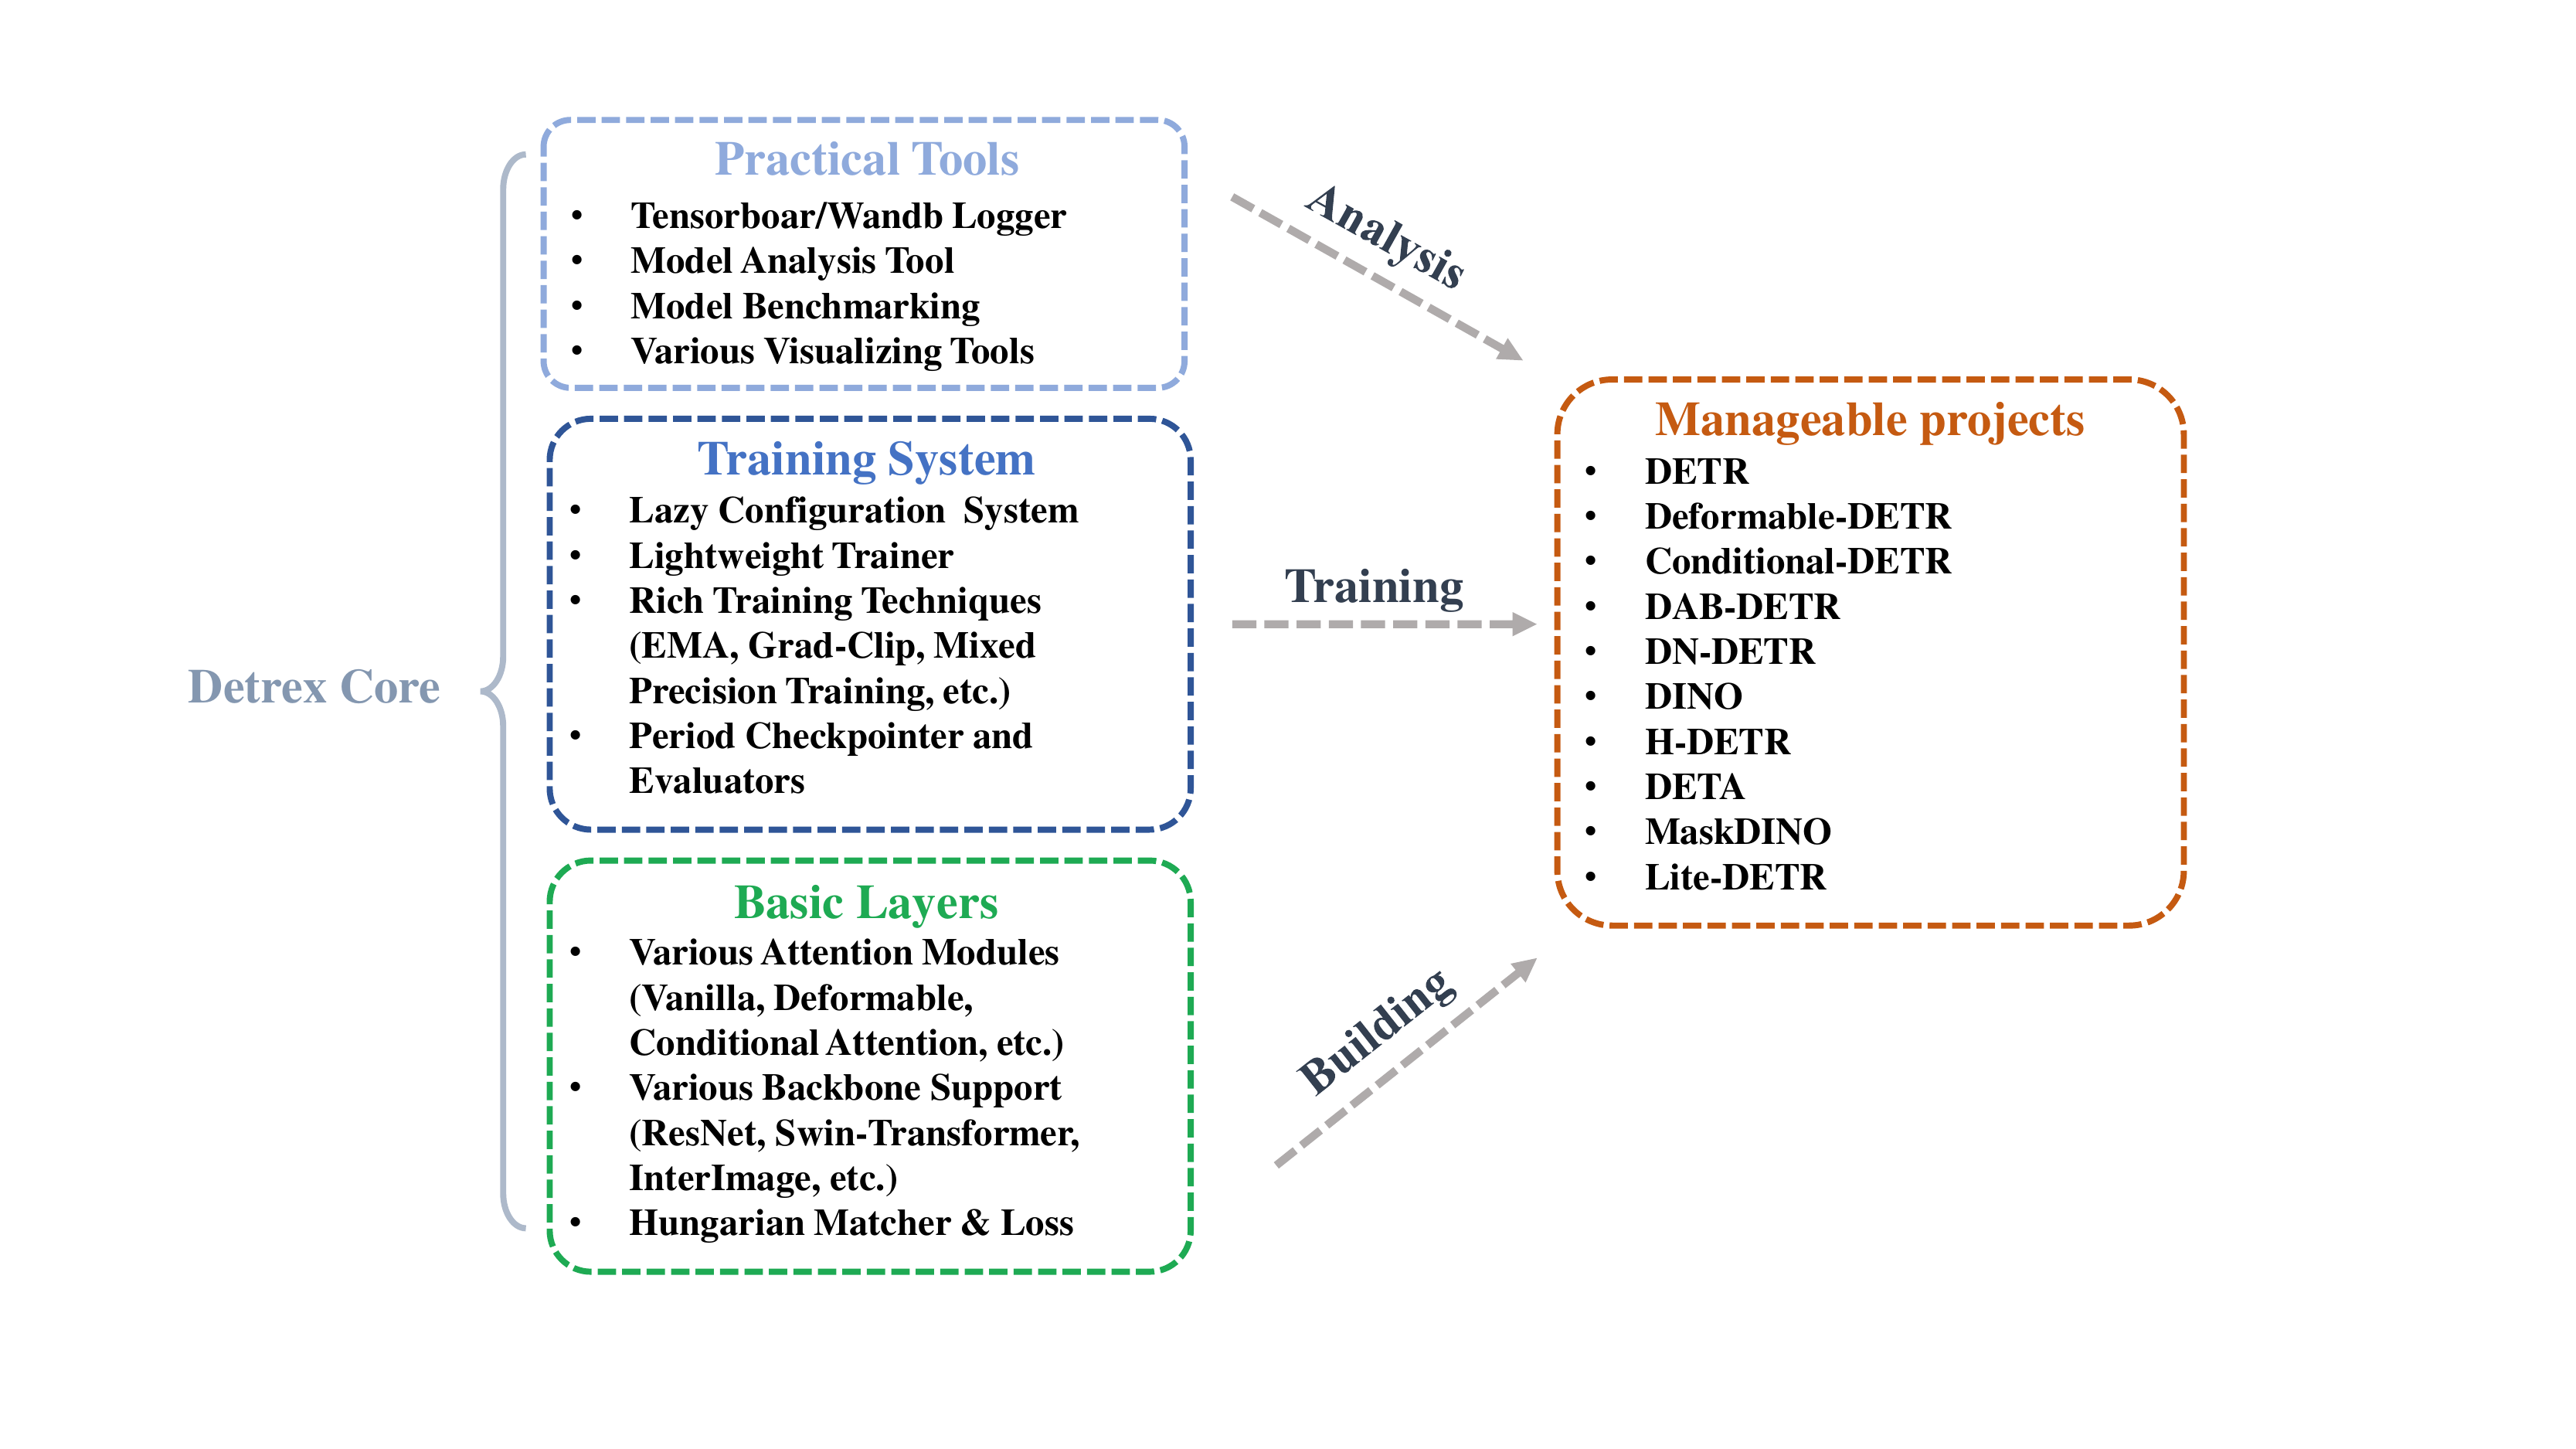}
    % \vspace{-0.1cm}
    \caption{The model design for detection transformers. 
    % \shilong{list all models.} 
    }
    \label{fig:detrex_design}
    % \vspace{-0.4cm}
\end{figure}

Optionally include extra information (complete proofs, additional experiments and plots) in the appendix.
This section will often be part of the supplemental material.
